# Supplementary material for: Is ChatGPT a Good Sentiment Analyzer? A Preliminary Study
Source: arXiv:2304.04339 source file (2024-02-17)
Supplement: Supplementary file 1 [file ECE-ECPE-prompts-appendix.tex]

\begin{table*}[th]

\centering
\scalebox{0.90}{
\begin{tabular}{l m{15cm}<{\centering}}
\toprule
\textbf{Task} & \textbf{Prompt}                                                                                                      \\ \midrule
ECE           & \begin{CJK}{UTF8}{gkai}
文档：\{\texttt{doc}\} \texttt{\textbackslash n} 以上文档的每一行代表一个子句，每行开头的数字表示该子句的编号。我们将包含情绪表达的子句称为``情绪子句''，将导致情绪发生的子句称为``原因子句''。我们注意到编号为 \{\texttt{emo\_id}\} 的子句 \{\texttt{emotion clause}\} 是情绪子句，情绪关键词是 \{\texttt{emotion}\} 。基于以上内容，分别完成以下任务。1. 用一句话描述编号为 \{\texttt{emo\_id}\} 的情绪子句对应的原因。2. 根据任务1的结果，输出原因子句的编号，你只需要找到最符合要求的那一个子句。3. 根据任务2的结果，将具有因果关系的子句匹配成(情绪子句编号，原因子句编号)的形式，最后将所有的编号配对按照集合的形式输出，例如\{(1,2),(3,4)\}。注意：情绪子句和原因子句有可能是同一个子句，且最终只需要输出情绪和原因最明显的配对。 

\end{CJK}
\\ 
ECPE          &  \begin{CJK}{UTF8}{gkai}
文档：\{\texttt{doc}\} \texttt{\textbackslash n} 以上文档的每一行代表一个子句，每行开头的数字表示该子句的编号。我们将包含情绪表达的子句称为``情绪子句''，将导致情绪发生的子句称为``原因子句''。基于以上内容，分别完成以下任务。1. 用一句话描述以上文档中包含的情绪以及它对应的原因。2. 输出任务1中情绪子句的编号，你只需要找到情绪强度最强的那一个子句。3.对于任务2中的每个情绪子句，找到导致其情绪的原因子句，并输出原因子句的编号，你只需要找到最符合要求的那一个子句。4.将以上具有因果关系的子句匹配成'(情绪子句编号，原因子句编号)'的形式，最后将所有的编号配对按照集合的形式输出，例如\{(1,2),(3,4)\}。注意：情绪子句和原因子句有可能是同一个子句，且最终只需要输出情绪和原因最明显的配对。 
\end{CJK}
\\ \bottomrule
\end{tabular}}
\caption{The prompts used for prompting ChatGPT on ECE and ECPE.}
\label{appendix-tab:ece-ecpe-prompt}
\end{table*}
